# Supplementary material for: Randomness In Neural Network Training: Characterizing The Impact of Tooling
Source: arXiv:2106.11872 source file (2021-06-22)
Supplement: Supplementary file 1 [file appendix.tex]

\appendix
\section{Appendix}
\subsection{Small CNN Architecture}
Optionally include extra information (complete proofs, additional experiments and plots) in the appendix.
This section will often be part of the supplemental material.
